# Supplementary material for: Consistent View Synthesis with Pose-Guided Diffusion Models
Source: arXiv:2303.17598 source file (2023-03-30)
Supplement: Supplementary file 1 [file fig_qualitative_supp.tex]

\begin{figure*}[t]
\centering
\includegraphics[width=0.9\linewidth]{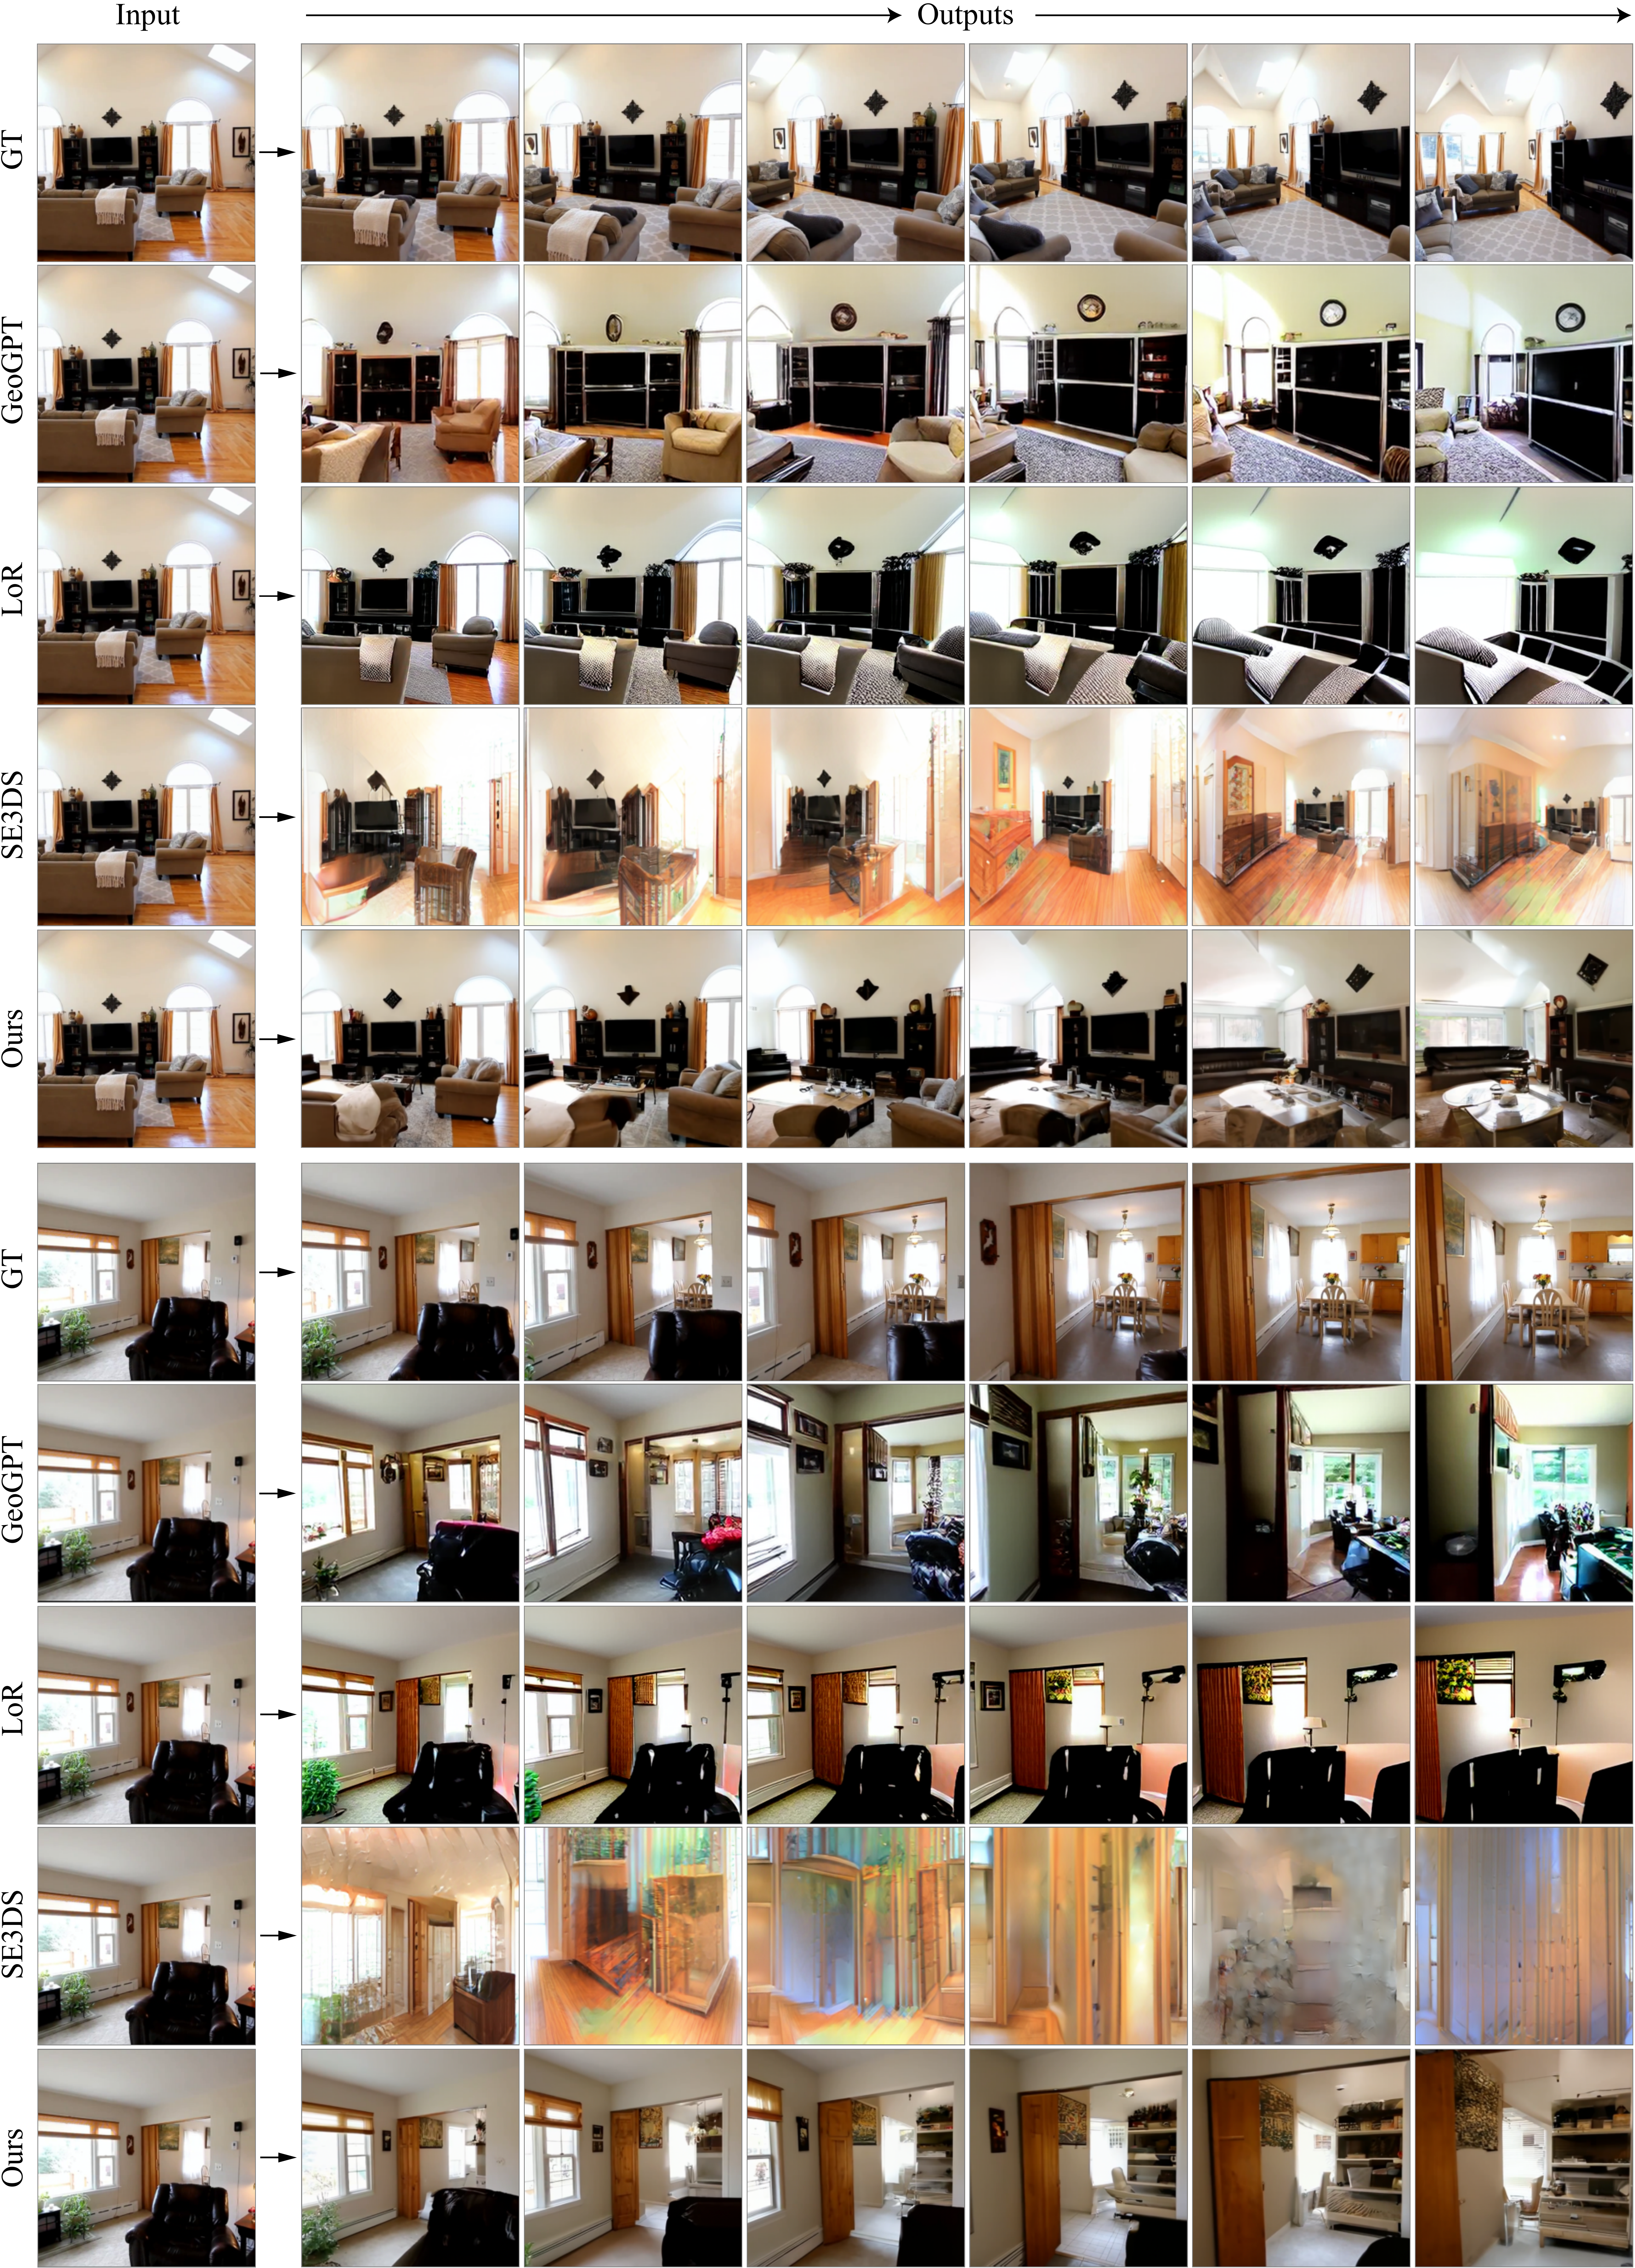}
\vspace{-3mm}
\caption{\textbf{Qualitative comparisons.} We present the additional long-term single-image view synthesis results, corresponding to Figure 5 in our main paper. 
}
\label{fig:additional_qualitative}
\end{figure*}
